# Supplementary material for: Fine-Grained Egocentric Hand-Object Segmentation: Dataset, Model, and Applications
Source: arXiv:2208.03826 source file (2022-08-07)
Supplement: Supplementary file 1 [file handobj_segmentation_supp.tex]

\begin{table*}[h!]
 \vspace{-17 pt}
    \begin{center}
     \resizebox{\textwidth}{!}{
      \begin{tabular}
      {l|c|c|c|c|c}
        \toprule % <-- Toprule here
        \textbf{Models} & \ Left Hand & \ Right Hand & \ Left-Hand Object & \ Right-Hand Object & \ Two-Hand Object \\
        \bottomrule % <-- Midrule here
        100-DOH \cite{shan2020understanding}  + PointRend \cite{kirillov2020pointrend} & - & - & 5.76 & 9.03 & 21.93  \\
        \midrule % <-- Midrule here
        Para. Decode & 83.58 & 83.48 & 43.03 & 26.12 & 40.18  \\
        \midrule
         Para. Decode + CCDA & 86.41 & 85.98 & 53.16 & 36.92 & 44.50  \\
        \midrule
        Seq. Decode & 84.17 & 84.15 & 41.52 & 27.47 & 30.56 \\
        \midrule
        Seq. Decode + CCDA & 83.86 & 84.02 & 50.27 &  28.12&  37.43 \\
        \midrule
        Seq. Decode + CB & 82.82 & 83.59 & 41.93 & 24.77 & 32.72  \\
        \midrule
        Seq. Decode + CB + CCDA & 84.11 & 83.85 & 49.93 & 29.13 & 41.29 \\
        \bottomrule % <-- Bottomrule here
      \end{tabular}
      }
      \vspace{2 pt}
      \caption{A quantitative evaluation on the hand-object segmentation on the out-of-the-distribution YouTube data. }
      \label{tab:handobj_segmentation}
    \end{center}
    \vspace{-29 pt}
\end{table*}
